# Supplementary material for: Handling abort commands for household kitchen robots
Source: arXiv:2408.14480 source file (2024-08-16)
Supplement: Supplementary file 1 [file appendix.tex]

Computational propaganda 

 Machine Common Sense (MCS)
 
\da{SUMO: analiza a lui SUMO.2-3 articole pe common sense reasoning cu SUMO. Be able to query SUMO.}

\da{Adam Pease-SUMO}

\da{Running Scenario: Wellness, i.e. dieta si sport}

SUMO is  expressed in SUO-KIF (Standard Upper Ontology Knowledge Interchange Format,  which  is  a  dialect  of  KIF (Knowledge  Interchange  Format)
Since KIF and SUO-KIF go beyond FOL and, SUMO axioms cannot be directly used by FOL reasoners.
 Adimen-SUMO v2.6, which is freely available at https://adimen.si.ehu.es/web/AdimenSUMO. 

"Fake News" cu generative models/Chat GPT
\subsection{Knowledge graphs for common sense reasoning}
COMET or ATOMIC vs SUMO pt Commonsense

SUMO

Fack checkers

\cite{thorne2018fever} FEVER dataset for fack verification

\subsection{Fake news datasets}
Kaggle Fake  News - 20,387 news items,

CoAID - COVID-19  healthcare  misinformation,  : 5251 news items.

\section{Common sense reasoning for fake news}

\subsection{Design patterns for fake news}
the ontology of fake news 

https://firstdraftnews.org/articles/fake-news-complicated/

\subsection{Cognitive biases for fake news}

\subsection{Defending against neural fake news}
Large language models for fake news
~\cite{zellers2019defending}

Tools that generate neural fake news: Grover\footnote{\url{https://thegradient.pub/why-we-released-grover/}}

\subsection{Tools for knowledge extraction from text}
\ag{De investigat cat de bine poate GPT translata text in formatul SUMO-KIF.}

\ag{SUMO are un translator basic din NLP2SUMO}

TEXT2KG

Newspaper Python library t
\subsection{Automatic Debunking}
Automatic counter speech generation

\subsection{Running scenario - Diet}
Wellnes, Sport

\subsubsection{Dataset}
~\cite{davis2023benchmarks}

Generare de neural fake news pe domeniul ales:

TRANSOMCS
